# Supplementary material for: Global Counterfactual Explainer for Graph Neural Networks
Source: arXiv:2210.11695 source file (2022-11-11)
Supplement: Supplementary file 1 [file sec_appendix.tex]

\section{Appendix}

\subsection{\label{sec:cost_aggregation_study}Recourse Cost Aggregation Study}

Recourse cost summation over original graphs may include outliers. Thus, we explore different aggregations from the recourse costs. The results from Table \ref{tab:quality_methods} shows median recourse cost, and Table \ref{tab:cost_aggregation} shows different metrics including $25\%$, $75\%$ percentiles, and \textbf{mean}. Note that the $50\%$ percentile is the same as the median which is shown in Table \ref{tab:quality_methods}. \name consistently outperforms competing baselines almost for all different aggregations of costs and datasets. Interestingly, the median is smaller than the mean cost for all cases, which suggests that there are original graphs far away from the summary counterfactual graphs and hard to be covered. Even in some cases, the difference is substantial. For \name, Mutagenicity has a 0.1135 median cost, whereas the mean cost is 0.1412, with a $24\%$ increase. We observe the same issue for other datasets and methods with different rates.

\begin{table*}[ht]
\centering
\caption{Different recourse cost (lower is better) aggregations for all methods and datasets. The used counterfactual summary and the setting are the same as Table \ref{tab:quality_methods}. The best is bold and the second best is underlined for each method and aggregation. GCFExplainer consistently outperforms competing baselines except in some rare cases, where our algorithm is still comparable to baselines.}
\begin{tabular}{ccccccccccccc}%
\toprule
& \multicolumn{3}{c}{\textbf{NCI1}} & \multicolumn{3}{c}{\textbf{Mutagenicity}} & \multicolumn{3}{c}{\textbf{AIDS}} & \multicolumn{3}{c}{\textbf{Proteins}} \\
& $25\%$ & $75\%$ & mean & 
$25\%$ & $75\%$ & mean & 
$25\%$ & $75\%$ & mean &
$25\%$ & $75\%$ & mean \\
\midrule
\textbf{Ground-Truth} & 
\underline{0.1095} & 0.1607 & 0.1484 &
0.0961 & \underline{0.1776} & \underline{0.1499} &
0.1689 & 0.2460 & 0.2180 &
\underline{0.1520} & 0.2985 & 0.2346 \\
\textbf{RCExplainer \cite{bajaj2021robust}} & 
0.1131 & 0.1712 & 0.1563 &
\underline{0.0922} & 0.1832 & 0.1560 &
\underline{0.1229} & \textbf{0.1921} & \textbf{0.1688} &
0.1756 & \underline{0.2814} & \underline{0.2306} \\
\textbf{CFF \cite{tan2022learning}} & 0.1100 & \underline{0.1532} & \underline{0.1375} &
0.0943 & 0.1814 & 0.1578 &
0.1382 & \underline{0.2004} & 0.1785 &
0.2058 & 0.3593 & 0.2901 \\
\textbf{GCFExplainer (Ours)} & 
\textbf{0.0975} & \textbf{0.1485} & \textbf{0.1294} &
\textbf{0.0899} & \textbf{0.1582} & \textbf{0.1412} &
\textbf{0.1182} & 0.2028 & \underline{0.1694} &
\textbf{0.1383} & \textbf{0.2639} & \textbf{0.2090} \\
\bottomrule
\end{tabular}
\label{tab:cost_aggregation}

\end{table*}
